# Supplementary material for: Compact Answers to Temporal Path Queries
Source: arXiv:2507.22143 source file (2025-07-29)
Supplement: Supplementary file 1 [file proof_data_hardness.tex]

Let $\TRPQ$ denote the language of TRPQs, as defined by the grammar provided in the article.
We partition this language into $\{\TRPQ_{\le k} \mid k \in \nn\}$,
where $\TRPQ_{\le k}$ is the set of queries with at most $k$ nested occurrences of the ``$?$'' operator.\\
Formally,
we define the \emph{rank} of a TRPQ $q$ inductively as follows:
\begin{itemize}
\item  if $q$ does not contain the ``$?$'' operator, then $q$ has rank $0$,
\item  if $q$ is of the form ``$?q'$'', then $q$ has rank $k+1$, where $k$ is the rank of $q'$,
\item  otherwise the rank of $q$ is the highest rank of any (strict) subquery of $q$.
\end{itemize}
And we define $\TRPQ_{\le k}$ as the set of all TRPQs with rank $\le k$.

We first show that for each $k \in \nn^+$, there is a fixed query $q \in \TRPQ_{\le k+1}$ s.t.~\pbma is hard for $\Sigma_k^P$ (resp. $\Pi_k^P$) if $k$ is odd (resp.~even).
Then we will lift this result to the $5$ problems for compact answers defined above.

The proof is a polynomial-time reduction from satisfiability of a quantified boolean formula in conjunctive normal form (CNF) with at most $k-1$ quantifier alternations, where the innermost quantifier is existential.
This problem is known to be complete for $\Sigma_k^P$ (resp. $\Pi_k^P$) if $k$ is odd (resp.~even).

We first illustrate the reduction, before giving a formal proof.
For simplicity, we start with boolean formulas with $0$ quantifier alternation.
In other words, we show that $\text{SAT}$ (where the formula is in CNF) can be reduced to an instance of $\pbma$ with a fixed TRPQ.\\

For readability, we will first illustrate the reduction with an abstract graph, and then only define the temporal graph used in our reduction, based on this graph.

Consider a boolean formula $\phi$ in CNF, of the form
\[\exists x_1, .., x_m. c_1 wedge .. \wedge c_n\]
where each $c_i$ is a boolean clause with variables in $\{x_1 .., x_m\}$.
We associate to $\phi$ a directed acyclic graph $G_\phi$ defined as follows.

The graph $G_\phi$ contains one ``source'' node $s$, and two nodes per variable $x_i$,
one for the literal $x_i$, and one for the literal $\neg x_i$.
The edges of this graph are $(s,x_1), (s, \neg x_1)$ and $\{x_i, \neg x_{i}\} \times \{x_{i+1}, \neg x_{i+1}\}$ for $i \in \{1, .., n-1\}$.\\
Each node in this graph is labeled with a subset of $\{0, .., n\}$.
Precisely, $s$ is labeled with the set $\{0, .., n\}$, and 
each literal is labeled with the set of indices of the clauses in which it does \emph{not} appear.\\

For instance, let
\[\phi = \exists x_1, x_2. (x_1 \vee x_2) \wedge (\neg x_2) \]
Then $G_\phi$ is the graph of Figure XXX.

It is easy to see that $\phi$ is satisfiable iff there exists path from $x_1$ or $\neg x_1$ to some node $n$ such that the intersection of all sets of indices on this path is the empty set.

More formally, let $\indexes{n}$ denote the set of indices labelling a node in $G_\phi$, and if $p = (n_1, .., n_k)$ is a path in $G_\phi$ (where each $n_i$ is a node), let
$\bigsqcap p$ denote the intersection of all sets opf labels along $p$, i.e.
$\bigsqcap p = \bigcap^k_{i = 1} \labels{n_i}$.

Then $\phi$ is satisfiable iff there is a path $p = (s, l_1, l_2, .., l_k)$ in $G_\phi$ with $k \ge 1$ s.t. $\bigsqcap p = \emptyset$.\\
Besides, observe that $\bigsqcap p = \emptyset$ iff $\bigscap (s, l_1, l_2, .., l_{k-1}) \cap \labels{l_k} = \emptyset$ (with $l_{k-1} = s$ for the limit case where $k = 1$).\\

Therefore 

\[\phi \te{is satisfiable iff there is a path} p = (s, l_1, l_2, .., l_k) \te{in} G_\phi \te{with} k \ge 1 \te{s.t.} \bigsqcap (s, l_1, l_2, .., l_{k-1}) \cap \labels{l_k} = \emptyset\]

This is the main intuition behind our reduction.
Precisely, we define a temporal graph $G$ a TRPQ $q$ and a tuple $\u \in XXX$ s.t. $\u \in $ iff this condition is verified.

The temporal graph $G = $ for the above formula is depicted in Figure XXX.

The nodes are identical to the nodes of $\G_\phi$, with the exception of an additional ``target'' node $t$.\\
The set of labels of each node is modeled at singleton intervals for the validity of some fixed predicate $a$.\\
For instance if $\labels{l} = \{1,2\}$ in $G_\phi$,
then $\val{} = XXX$.

Finally, an edges is labeled identically to its sources node, i.e.
XXXX

the 

us represent a path $p$ in this graph as a finite sequence of nodes, let us use $\labels{n}$ 

such that every two consecutive nodes are 

To complete the reduction, we show how this condition can be verified by transforming $G_\phi$ into a temporal graph $G'_\phi$, and evaluating a TRPQ $q$ over $G'_\phi$ that does not depend on $\phi$.

The temporal graph can be  obtained from $G_\phi$ as follows:

In this graph, each 
Eac

Besides, $t$ is labeled with the set of all clause indexes, i.e. with $\{1, .., n\}$,

variables $x_1, .., x_n$.
We associate an index to each clause in $\phi$.

We assume that clauses are indexed
one may associate the index $1$ with the first clause $(x_1 \vee x_2)$, and the index $2$ with the second clause $(\neg x_2)$.

For instance, if $\phi$ has two variables $x_1$ and $x_2$, then this graph is the one of Figure XXX.\\
In this graph, each path from $s$ to $t$ represents a valuation of the variable of $\phi$, and conversely.

Next, for each possible literal $l$,
we label the node that corresponds to $l$ with the set of indexes of the clauses in which $l$ does \emph{not} appear.

from:
\begin{itemize}
\item
\end{itemize}

The TRPQ for this case is
\[q_0 = \]

For any 
Consider the quantified boolean formula $\exists $   
%%% Local Variables:
%%% mode: latex
%%% TeX-master: "../../appendix"
%%% End:
