# Supplementary material for: Compact Answers to Temporal Path Queries
Source: arXiv:2507.22143 source file (2025-07-29)
Supplement: Supplementary file 2 [file finite.tex]

\section{Finiteness}
\label{sec:finite}

\subsection{in $\tuplest$}

\begin{proposition}
  Let $G = \tup{\tdg \fg, \valz}$ be a temporal graph over dense time, and let $q$ be a TRPQ such that $\delta$ is a singleton interval for every operator of the form $\tndelta$ in $q$.
  Then $\evalcit{q}$ is finite.
\end{proposition}
\begin{proof}
  Immediate from the definition of $\evalcit{q}$ and Proposition~\ref{prop:correct_t}.\\
  In particular, for the $[m,\_]$ operator, it is sufficient to observe that $\tdg$ is bounded, and that all operations on time points in the definition of $\evalcit{q}$ consist in adding or subtracting interval boundaries that are present in $G$ or $q$.
\end{proof}

%%% Local Variables:
%%% mode: latex
%%% TeX-master: "../../main"
%%% End:
